# Supplementary material for: Triton-distributed: Programming Overlapping Kernels on Distributed AI Systems with the Triton Compiler
Source: arXiv:2504.19442 source file (2025-06-05)
Supplement: Supplementary file 1 [file appendix.tex]

\section{Hello World}
%\subsection{Hello World}
